# Supplementary material for: An interpretable approach to automating the assessment of biofouling in video footage
Source: arXiv:2503.12875 source file (2025-03-31)
Supplement: Supplementary file 1 [file X_supp_cut.tex]

% ==================================================================================================================================
\FloatBarrier
\newpage
\section{Detecting paint damage}
% ==================================================================================================================================

\begin{table}[!b]
\caption{Antifoulant coating quality (PQ) scale.}
\label{tbl:coating_quality}
\begin{tabular}{l|p{13cm}}
\toprule
Rank & Description \\
\midrule
1 & Paint not present or in poor condition (16-100\% of surface scratched/corroded/fouled).  \\
2 & Paint visible and in fair condition or slightly obscured (1-15\% of surface scratched/corroded/fouled).  \\
3 & Paint visible and in good condition.  \\
\bottomrule
\end{tabular}
\end{table}

\begin{table*}[!h]
\caption[Brief summary of the 2021 cropped paint damage dataset.]{Brief summary of the 2021 cropped paint damage dataset. We show example training (first row) and testing (second row) images, and a table of the counts of each category in the dataset below. This dataset uses the same imagery as the 2021 cropped dataset. }
\label{tbl:dataset_2023_cropped_pq}
\centering
\includegraphics[width=1\textwidth]{dataset_summary/paintdamage_2021_cropped_training.jpg}
\includegraphics[width=1\textwidth]{dataset_summary/paintdamage_2021_cropped_test.jpg}
% \resizebox{\textwidth}{!}{%
\begin{tabular}[t]{lrrrr}
\toprule
\textbf{Category} & PQ 1 & PQ 2 & PQ 3 & Total \\
\midrule
\textbf{Training}  & 3464 & 3665 & 2293 & 9422  \\ 
\textbf{Test}  & 408  & 287 & 146 & 841 \\ 
\bottomrule
\end{tabular}%}
\end{table*}

\begin{figure*}[!b]
     \centering
     \begin{subfigure}[b]{0.3\textwidth}
         \centering
         \caption{Paint damage present}
         \label{fig:prototype_examples_pets_2}
         \includegraphics[width=\textwidth]{plots/2024_biofouling_prauc_paintdamage.png}
     \end{subfigure}%
     \begin{subfigure}[b]{0.09\textwidth}
         % \caption{No vessel hull present}
         \picdims[height=4.5cm]{\textwidth}{3.5cm}{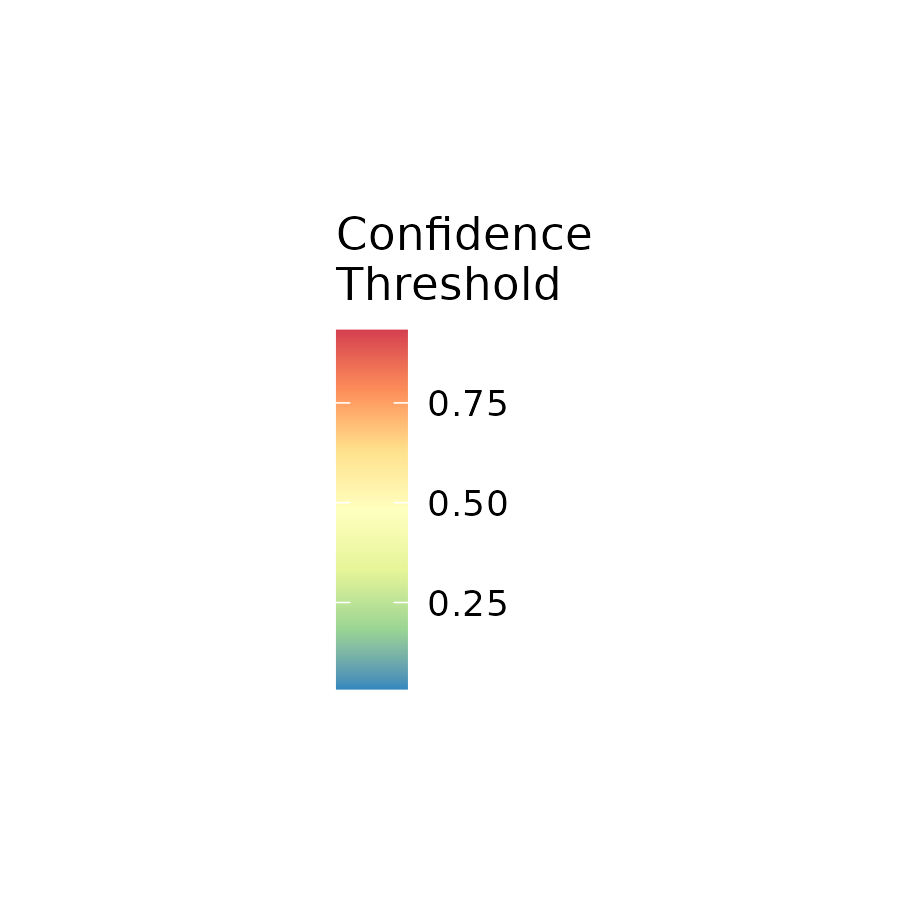}
         \vspace{1cm}
     \end{subfigure} \\
        \caption[Precision-recall curves for our best ComFe model for detecting the presence of fouling, paint damage and niche areas. ]{Precision-recall curves for our best ComFe model for detecting the presence of fouling, paint damage and niche areas, on the 2021 cropped test set. The models are trained using a ComFe head on the DINOv2 ViT-B/14 (f) w/reg backbone, using the 2021 cropped training data.}
        \label{fig:model_suite_average_precision}
\end{figure*}

\begin{figure*}[!tb]
     \centering
     \begin{subfigure}[b]{0.12\textwidth}
         \centering
        \begin{overpic}[height=\textwidth, width=\textwidth]{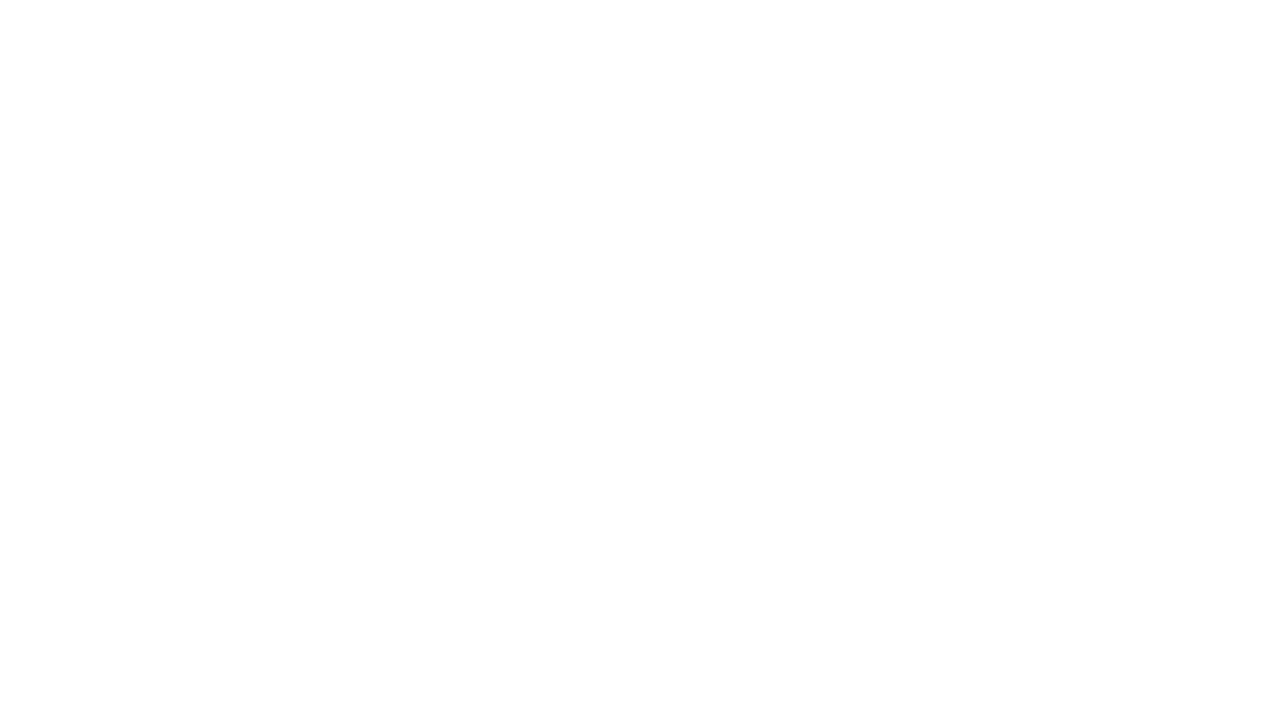}
         \put (0,50) {\parbox{2cm}{\centering Input image}}
        \end{overpic}
        \begin{overpic}[height=\textwidth, width=\textwidth]{example_images/1280px-HD_transparent_picture.png}
         \put (0,50) {\parbox{2cm}{\centering Class\\prediction}}
        \end{overpic}
        % \begin{overpic}[height=\textwidth, width=\textwidth]{example_images/1280px-HD_transparent_picture.png}
        %  \put (0,50) {\parbox{2cm}{\centering Image\\prototypes}}
        % \end{overpic}
     \end{subfigure}
     \begin{subfigure}[b]{0.12\textwidth}
         \centering
         \caption{Undamaged}
         \label{fig:prototype_examples_planes_2}
         \includegraphics[width=\textwidth]{figures/paint_damage/True_0_656_raw.jpg}
         \includegraphics[width=\textwidth]{figures/paint_damage/True_0_656_class.jpg}
     \end{subfigure}
     \begin{subfigure}[b]{0.12\textwidth}
         \centering
         \caption{Undamaged}
         \label{fig:prototype_examples_pets_2}
         \includegraphics[width=\textwidth]{figures/paint_damage/True_0_748_raw.jpg}
         \includegraphics[width=\textwidth]{figures/paint_damage/True_0_748_class.jpg}
     \end{subfigure}
     \begin{subfigure}[b]{0.12\textwidth}
         \centering
         \caption{Undamaged}
         \label{fig:prototype_examples_planes_1}
         \includegraphics[width=\textwidth]{figures/paint_damage/False_1_720_raw.jpg}
         \includegraphics[width=\textwidth]{figures/paint_damage/False_1_720_class.jpg}
     \end{subfigure}
     \begin{subfigure}[b]{0.12\textwidth}
         \centering
         \caption{Damaged}
         \label{fig:prototype_examples_cars_1}
         \includegraphics[width=\textwidth]{figures/paint_damage/False_1_115_raw.jpg}
         \includegraphics[width=\textwidth]{figures/paint_damage/False_1_115_class.jpg}
     \end{subfigure}
     \begin{subfigure}[b]{0.12\textwidth}
         \centering
         \caption{Damaged}
         \label{fig:prototype_examples_cars_2}
         \includegraphics[width=\textwidth]{figures/paint_damage/False_1_772_raw.jpg}
         \includegraphics[width=\textwidth]{figures/paint_damage/False_1_772_class.jpg}
     \end{subfigure}
     \begin{subfigure}[b]{0.12\textwidth}
         \centering
         \caption{Damaged}
         \label{fig:prototype_examples_pets_1}
         \includegraphics[width=\textwidth]{figures/paint_damage/False_1_12_raw.jpg}
         \includegraphics[width=\textwidth]{figures/paint_damage/False_1_12_class.jpg}
     \end{subfigure}
        \caption{Segmentation masks predicted by ComFe for the extent of paint damage. }
        \label{fig:salient_features_paintdamage}
\end{figure*}

\begin{figure*}[!tb]
     \centering
     \begin{subfigure}[b]{0.45\textwidth}
         \centering
         % \caption{Clean}
         % \label{fig:prototype_examples_pets_2}
         \includegraphics[width=\textwidth]{plots/2024_biofouling_paint_coverage.png}
     \end{subfigure}
        \caption{Predicted coverage within an image of fouling and paint damage by ComFe versus label categories for fouling and paint damage severity. }
        \label{fig:severity_coverage}
\end{figure*}

\begin{figure*}[!h]
     \centering
     \begin{subfigure}[b]{0.45\textwidth}
         \centering
         % \label{fig:prototype_examples_pets_2}
         \includegraphics[width=\textwidth]{figures-prototypes/paint_damage/class_prototype_0.jpg}
         \caption{No Paint Damage}
     \end{subfigure}%
     \hfill{}
     \begin{subfigure}[b]{0.45\textwidth}
         \centering
         % \label{fig:prototype_examples_pets_2}
         \includegraphics[width=\textwidth]{figures-prototypes/paint_damage/class_prototype_1.jpg}
         \caption{Paint Damage}
     \end{subfigure}
        \caption{Predicted coverage within an image of fouling and paint damage by ComFe versus label categories for fouling and paint damage severity. }
        \label{fig:severity_coverage}
\end{figure*}

\begin{figure*}[!t]
     \centering
     \begin{subfigure}[b]{0.11\textwidth}
         \centering
        \begin{overpic}[height=0.6\textwidth, width=\textwidth]{example_images/1280px-HD_transparent_picture.png}
         \put (0,20) {\parbox{1.5cm}{\centering \small Fouling}}
        \end{overpic}
        \begin{overpic}[height=0.6\textwidth, width=\textwidth]{example_images/1280px-HD_transparent_picture.png}
         \put (0,20) {\parbox{1.5cm}{\centering \small Paint\\Damage}}
        \end{overpic}
        \begin{overpic}[height=0.6\textwidth, width=\textwidth]{example_images/1280px-HD_transparent_picture.png}
         \put (0,20) {\parbox{1.5cm}{\centering \small No\\Concerns}}
        \end{overpic}
     \end{subfigure}%
     \begin{subfigure}[b]{0.11\textwidth}
         \centering
         \includegraphics[width=\textwidth]{figures-video/day2-4.mkv/frames/fouling_present/Frame-1386}
         \includegraphics[width=\textwidth]{figures-video/day2-4.mkv/frames/paint_damaged/Frame-1482}
         \includegraphics[width=\textwidth]{figures-video/day2-4.mkv/frames/no_damage_fouling/Frame-804}
     \end{subfigure}%
     \begin{subfigure}[b]{0.11\textwidth}
         \centering
         \includegraphics[width=\textwidth]{figures-video/day2-4.mkv/frames/fouling_present/Frame-1842}
         \includegraphics[width=\textwidth]{figures-video/day2-4.mkv/frames/paint_damaged/Frame-5826}
         \includegraphics[width=\textwidth]{figures-video/day2-4.mkv/frames/no_damage_fouling/Frame-4944}
     \end{subfigure}%
     \begin{subfigure}[b]{0.11\textwidth}
         \centering
         \includegraphics[width=\textwidth]{figures-video/day2-4.mkv/frames/fouling_present/Frame-2100}
         \includegraphics[width=\textwidth]{figures-video/day2-4.mkv/frames/paint_damaged/Frame-6642}
         \includegraphics[width=\textwidth]{figures-video/day2-4.mkv/frames/no_damage_fouling/Frame-6207}
     \end{subfigure}%
     \begin{subfigure}[b]{0.11\textwidth}
         \centering
         \includegraphics[width=\textwidth]{figures-video/day2-4.mkv/frames/fouling_present/Frame-3156}
         \includegraphics[width=\textwidth]{figures-video/day2-4.mkv/frames/paint_damaged/Frame-8271}
         \includegraphics[width=\textwidth]{figures-video/day2-4.mkv/frames/no_damage_fouling/Frame-7284}
     \end{subfigure}%
     \begin{subfigure}[b]{0.11\textwidth}
         \centering
         \includegraphics[width=\textwidth]{figures-video/day2-4.mkv/frames/fouling_present/Frame-3339}
         \includegraphics[width=\textwidth]{figures-video/day2-4.mkv/frames/paint_damaged/Frame-8859}
         \includegraphics[width=\textwidth]{figures-video/day2-4.mkv/frames/no_damage_fouling/Frame-10542}
     \end{subfigure}%
     \begin{subfigure}[b]{0.11\textwidth}
         \centering
         \includegraphics[width=\textwidth]{figures-video/day2-4.mkv/frames/fouling_present/Frame-4857}
         \includegraphics[width=\textwidth]{figures-video/day2-4.mkv/frames/paint_damaged/Frame-9585}
         \includegraphics[width=\textwidth]{figures-video/day2-4.mkv/frames/no_damage_fouling/Frame-12453}
     \end{subfigure}%
     \begin{subfigure}[b]{0.11\textwidth}
         \centering
         \includegraphics[width=\textwidth]{figures-video/day2-4.mkv/frames/fouling_present/Frame-6882}
         \includegraphics[width=\textwidth]{figures-video/day2-4.mkv/frames/paint_damaged/Frame-11808}
         \includegraphics[width=\textwidth]{figures-video/day2-4.mkv/frames/no_damage_fouling/Frame-13212}
     \end{subfigure}%
     \begin{subfigure}[b]{0.11\textwidth}
         \centering
         \includegraphics[width=\textwidth]{figures-video/day2-4.mkv/frames/fouling_present/Frame-9948}
         \includegraphics[width=\textwidth]{figures-video/day2-4.mkv/frames/paint_damaged/Frame-19497}
         \includegraphics[width=\textwidth]{figures-video/day2-4.mkv/frames/no_damage_fouling/Frame-19422}
     \end{subfigure}\\
     % ==================================================================================
     \begin{subfigure}[b]{1\textwidth}
         \centering
         \includegraphics[width=\textwidth]{figures-video/day2-4.mkv/plots/biofouling_paint_all-plot-smoothed.png}
     \end{subfigure}
        \caption[Analysis of ROV captured video with heavy fouling for macrofouling and paint damage.]{Analysis of ROV captured video with heavy fouling for macrofouling and paint damage. The dots in the timeseries represent the frames shown above the plot, which are selected using an automated procedure. The dashed lines represent the proportion of fouling or paint damage coverage identified with the model, and the horizontal lines show the thresholds used to classify frames as having paint damage or macrofouling present.}
        \label{fig:exec_video_trial_examples_heavy_fouling}
\end{figure*}

\begin{figure*}[!h]
     \centering
     \begin{subfigure}[b]{0.11\textwidth}
         \centering
        \begin{overpic}[height=0.6\textwidth, width=\textwidth]{example_images/1280px-HD_transparent_picture.png}
         \put (0,20) {\parbox{1.5cm}{\centering \small Fouling}}
        \end{overpic}
        \begin{overpic}[height=0.6\textwidth, width=\textwidth]{example_images/1280px-HD_transparent_picture.png}
         \put (0,20) {\parbox{1.5cm}{\centering \small Paint\\Damage}}
        \end{overpic}
        \begin{overpic}[height=0.6\textwidth, width=\textwidth]{example_images/1280px-HD_transparent_picture.png}
         \put (0,20) {\parbox{1.5cm}{\centering \small No\\Concerns}}
        \end{overpic}
     \end{subfigure}%
     \begin{subfigure}[b]{0.11\textwidth}
         \centering
         \includegraphics[width=\textwidth]{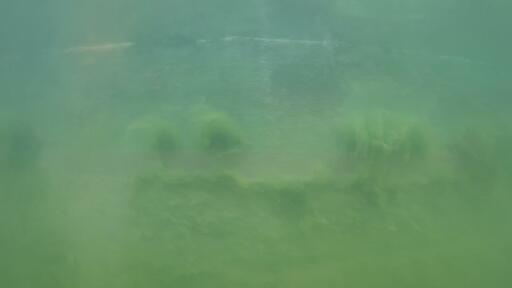}
         \includegraphics[width=\textwidth]{figures-video/day2-2.mkv/frames/paint_damaged/Frame-5718}
         \includegraphics[width=\textwidth]{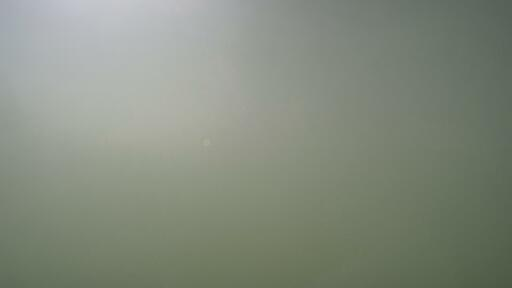}
     \end{subfigure}%
     \begin{subfigure}[b]{0.11\textwidth}
         \centering
         \includegraphics[width=\textwidth]{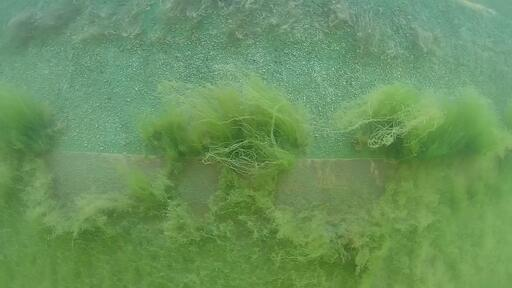}
         \includegraphics[width=\textwidth]{figures-video/day2-2.mkv/frames/paint_damaged/Frame-7323}
         \includegraphics[width=\textwidth]{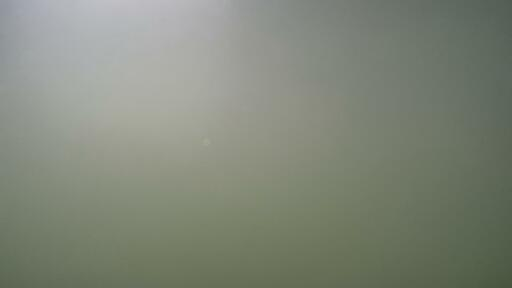}
     \end{subfigure}%
     \begin{subfigure}[b]{0.11\textwidth}
         \centering
         \includegraphics[width=\textwidth]{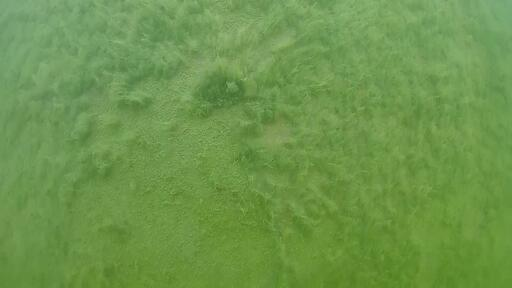}
         \includegraphics[width=\textwidth]{figures-video/day2-2.mkv/frames/paint_damaged/Frame-10032}
         \includegraphics[width=\textwidth]{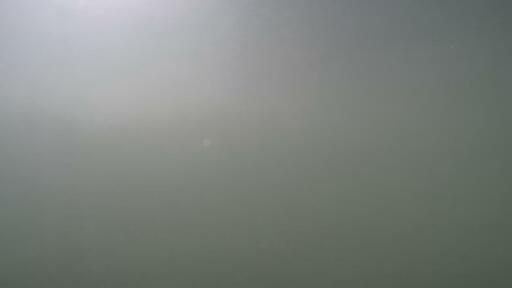}
     \end{subfigure}%
     \begin{subfigure}[b]{0.11\textwidth}
         \centering
         \includegraphics[width=\textwidth]{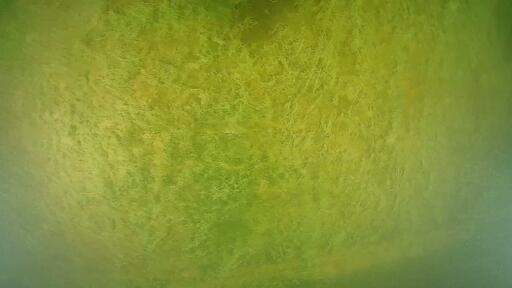}
         \includegraphics[width=\textwidth]{figures-video/day2-2.mkv/frames/paint_damaged/Frame-12405}
         \includegraphics[width=\textwidth]{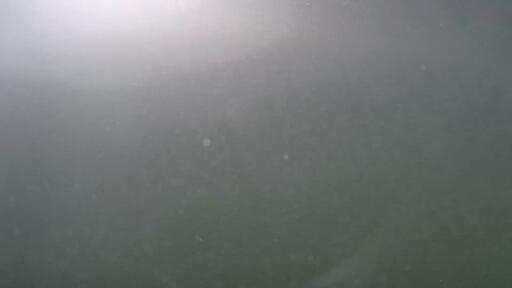}
     \end{subfigure}%
     \begin{subfigure}[b]{0.11\textwidth}
         \centering
         \includegraphics[width=\textwidth]{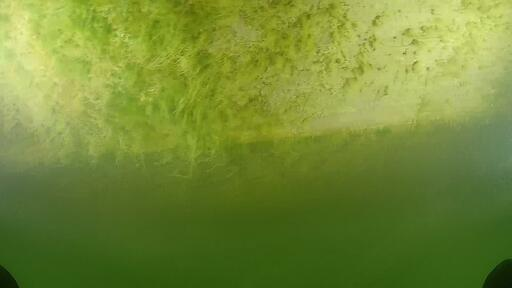}
         \includegraphics[width=\textwidth]{figures-video/day2-2.mkv/frames/paint_damaged/Frame-15372}
         \includegraphics[width=\textwidth]{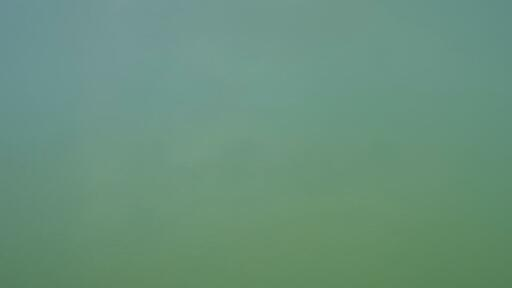}
     \end{subfigure}%
     \begin{subfigure}[b]{0.11\textwidth}
         \centering
         \includegraphics[width=\textwidth]{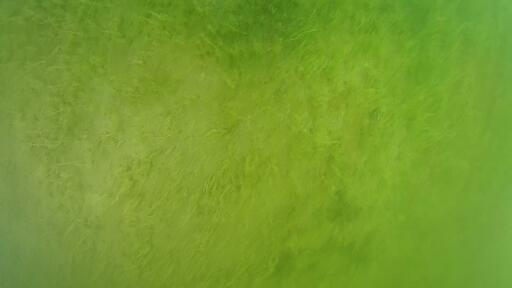}
         \includegraphics[width=\textwidth]{figures-video/day2-2.mkv/frames/paint_damaged/Frame-15795}
         \includegraphics[width=\textwidth]{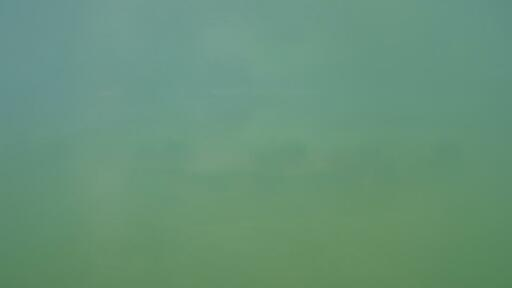}
     \end{subfigure}%
     \begin{subfigure}[b]{0.11\textwidth}
         \centering
         \includegraphics[width=\textwidth]{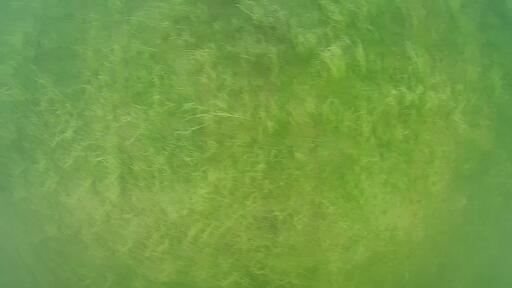}
         \includegraphics[width=\textwidth]{figures-video/day2-2.mkv/frames/paint_damaged/Frame-23094}
         \includegraphics[width=\textwidth]{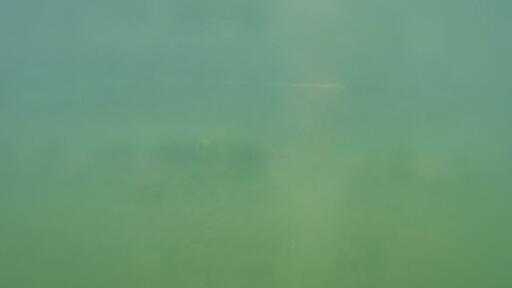}
     \end{subfigure}%
     \begin{subfigure}[b]{0.11\textwidth}
         \centering
         \includegraphics[width=\textwidth]{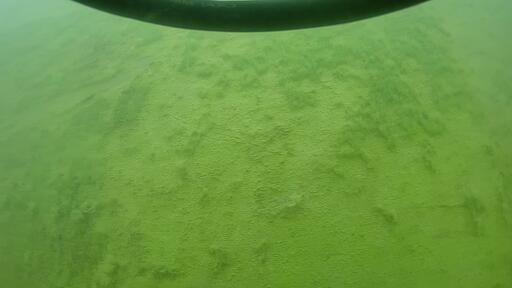}
         \includegraphics[width=\textwidth]{figures-video/day2-2.mkv/frames/paint_damaged/Frame-25587}
         \includegraphics[width=\textwidth]{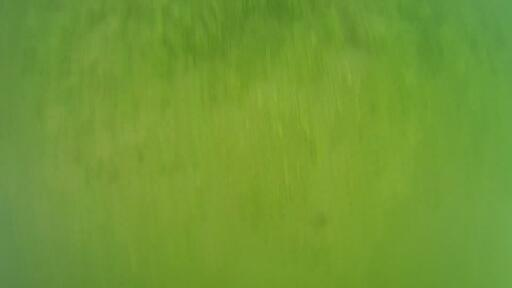}
     \end{subfigure}\\
     % ==================================================================================
     \begin{subfigure}[b]{1\textwidth}
         \centering
         \includegraphics[width=\textwidth]{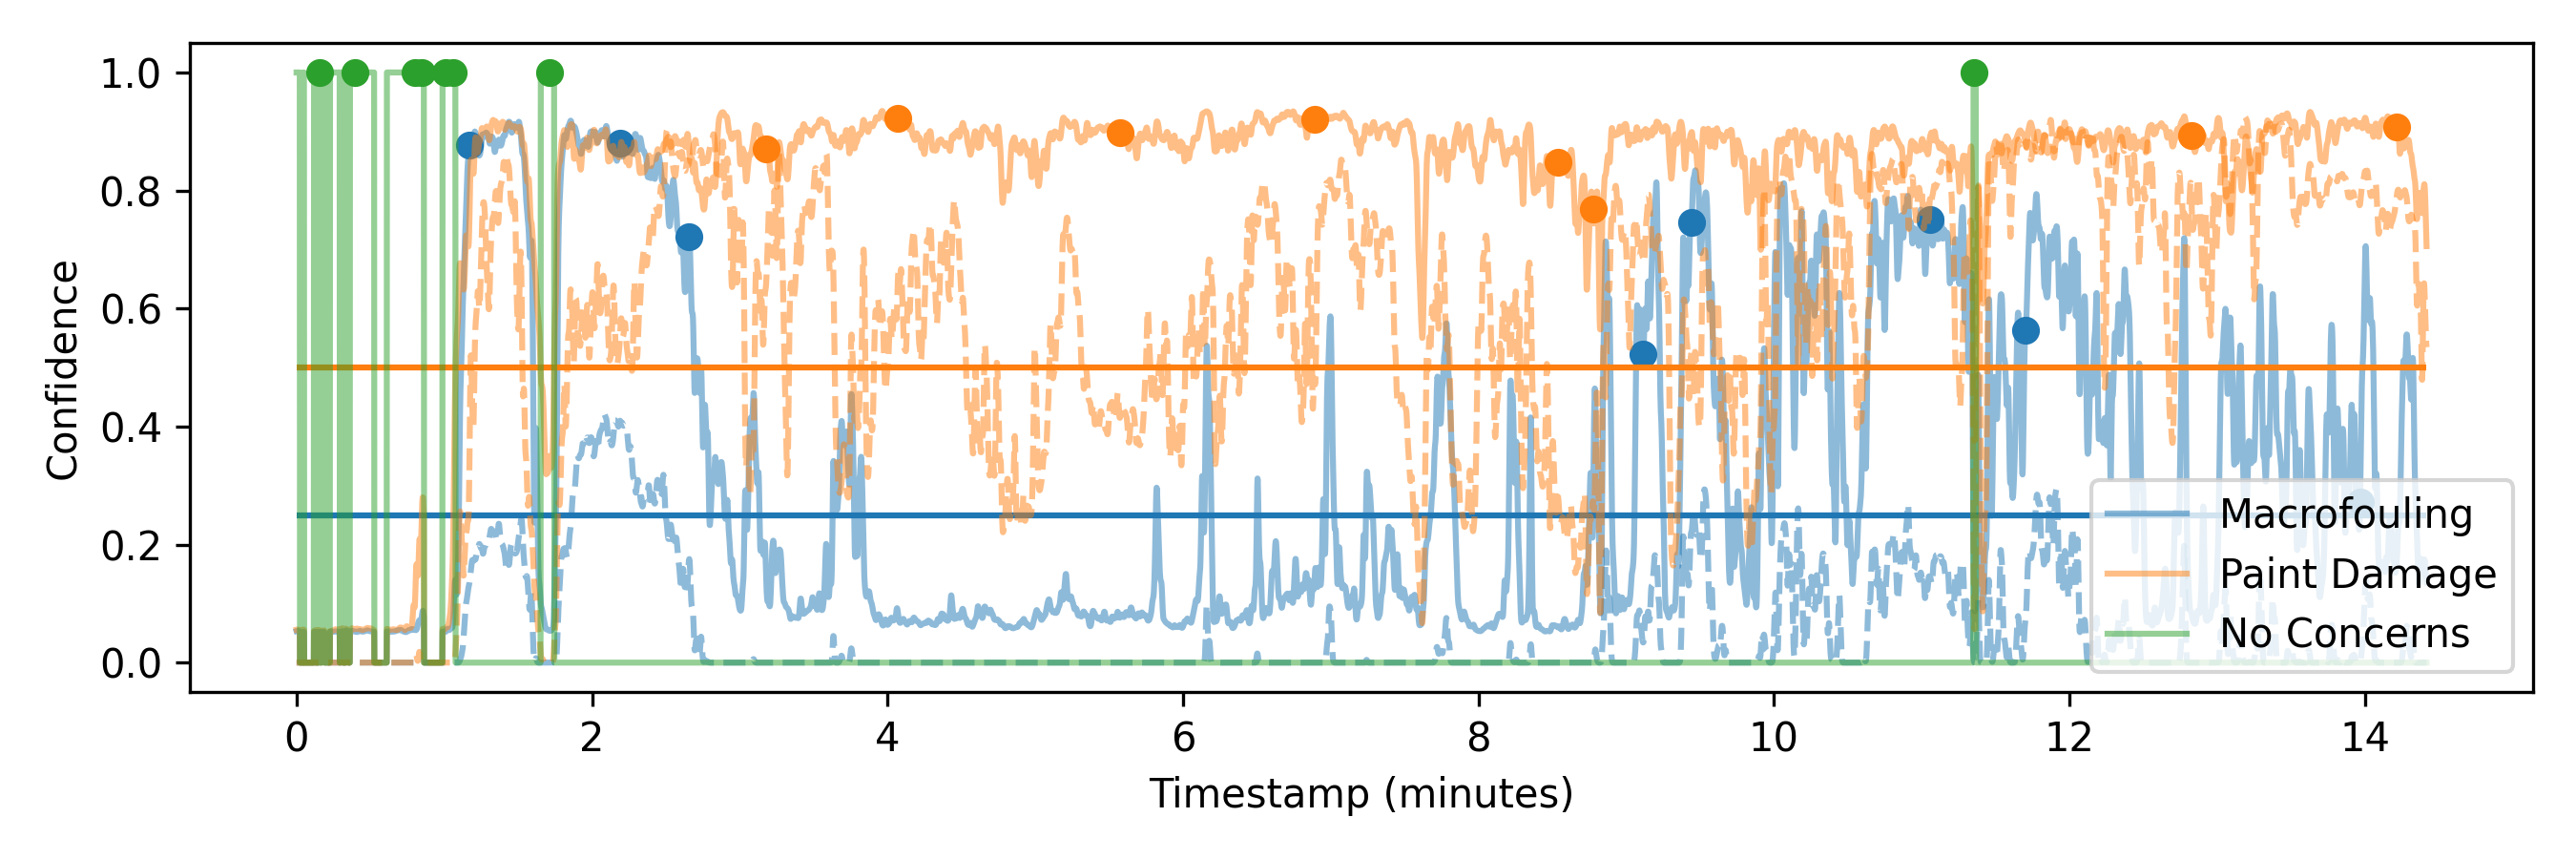}
     \end{subfigure}
        \caption[Analysis of ROV captured video with heavy fouling for macrofouling and paint damage using the ComFe model.]{Analysis of ROV captured video with heavy fouling for macrofouling and paint damage using the ComFe model. The dots in the timeseries represent the frames shown above the plot, which are selected using the SKMPS method. The dashed lines represent the proportion of fouling or paint damage coverage predicted by the ComFe head, and the horizontal lines show the thresholds used to classify frames as having paint damage or macrofouling present.}
        \label{fig:video_trial_examples_heavy_fouling}
\end{figure*}

\begin{figure*}[!h]
     \centering
     \begin{subfigure}[b]{0.11\textwidth}
         \centering
        \begin{overpic}[height=0.6\textwidth, width=\textwidth]{example_images/1280px-HD_transparent_picture.png}
         \put (0,20) {\parbox{1.5cm}{\centering \small Fouling}}
        \end{overpic}
        \begin{overpic}[height=0.6\textwidth, width=\textwidth]{example_images/1280px-HD_transparent_picture.png}
         \put (0,20) {\parbox{1.5cm}{\centering \small Paint\\Damage}}
        \end{overpic}
        \begin{overpic}[height=0.6\textwidth, width=\textwidth]{example_images/1280px-HD_transparent_picture.png}
         \put (0,20) {\parbox{1.5cm}{\centering \small No\\Concerns}}
        \end{overpic}
     \end{subfigure}%
     \begin{subfigure}[b]{0.11\textwidth}
         \centering
         \includegraphics[width=\textwidth]{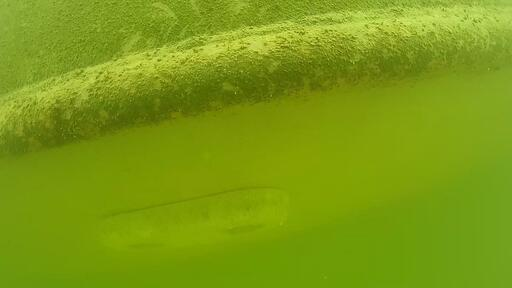}
         \includegraphics[width=\textwidth]{figures-video/day1-4.mkv/frames/paint_damaged/Frame-3729}
         \includegraphics[width=\textwidth]{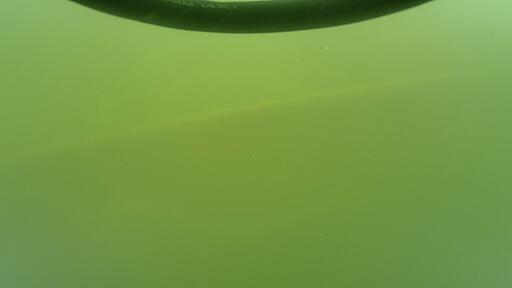}
     \end{subfigure}%
     \begin{subfigure}[b]{0.11\textwidth}
         \centering
         \includegraphics[width=\textwidth]{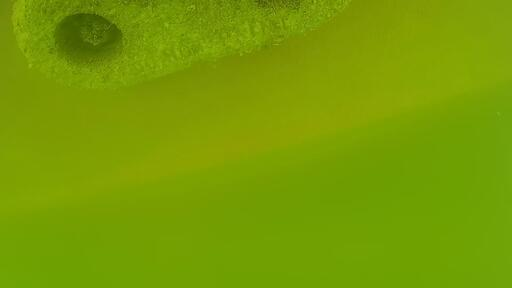}
         \includegraphics[width=\textwidth]{figures-video/day1-4.mkv/frames/paint_damaged/Frame-4188}
         \includegraphics[width=\textwidth]{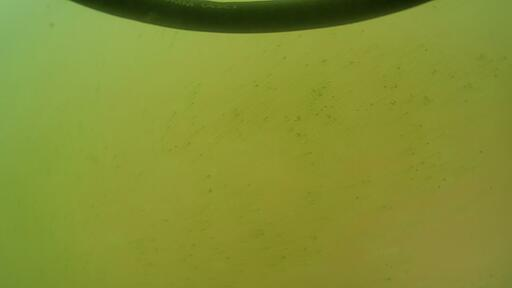}
     \end{subfigure}%
     \begin{subfigure}[b]{0.11\textwidth}
         \centering
         \includegraphics[width=\textwidth]{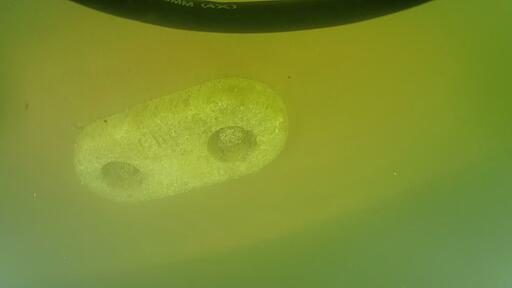}
         \includegraphics[width=\textwidth]{figures-video/day1-4.mkv/frames/paint_damaged/Frame-6096}
         \includegraphics[width=\textwidth]{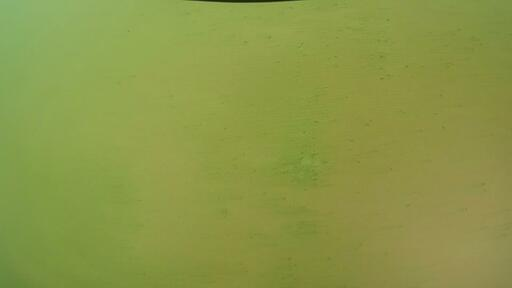}
     \end{subfigure}%
     \begin{subfigure}[b]{0.11\textwidth}
         \centering
         \includegraphics[width=\textwidth]{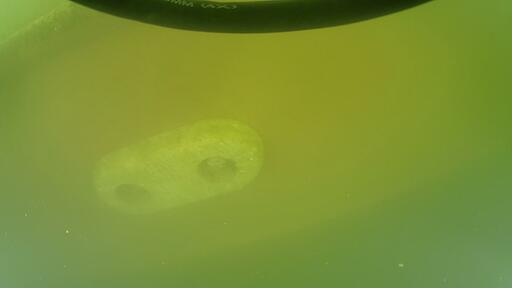}
         \includegraphics[width=\textwidth]{figures-video/day1-4.mkv/frames/paint_damaged/Frame-8394}
         \includegraphics[width=\textwidth]{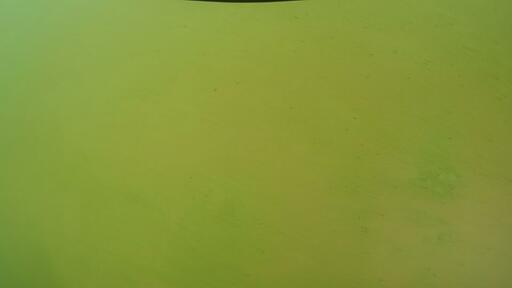}
     \end{subfigure}%
     \begin{subfigure}[b]{0.11\textwidth}
         \centering
         \includegraphics[width=\textwidth]{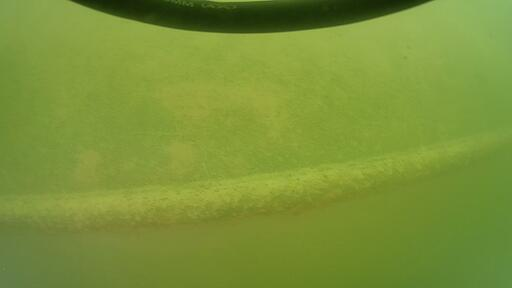}
         \includegraphics[width=\textwidth]{figures-video/day1-4.mkv/frames/paint_damaged/Frame-13059}
         \includegraphics[width=\textwidth]{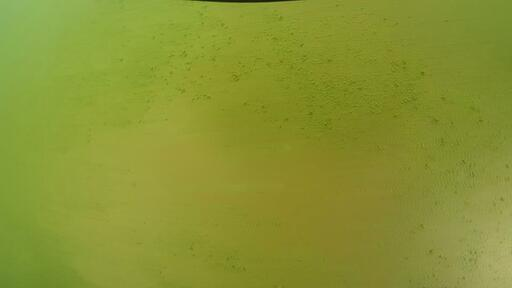}
     \end{subfigure}%
     \begin{subfigure}[b]{0.11\textwidth}
         \centering
         \includegraphics[width=\textwidth]{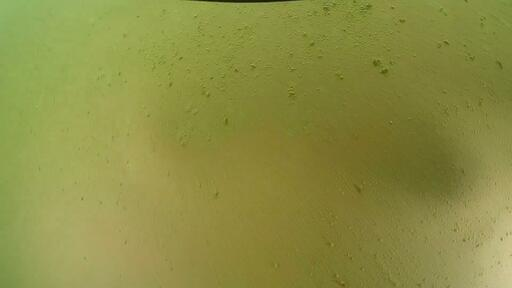}
         \includegraphics[width=\textwidth]{figures-video/day1-4.mkv/frames/paint_damaged/Frame-13431}
         \includegraphics[width=\textwidth]{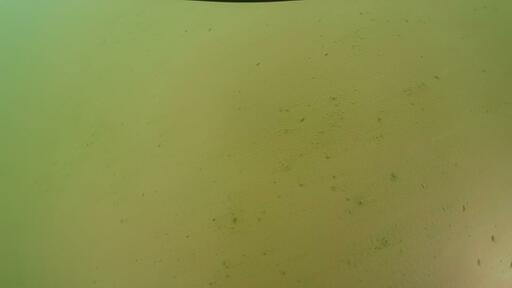}
     \end{subfigure}%
     \begin{subfigure}[b]{0.11\textwidth}
         \centering
         \includegraphics[width=\textwidth]{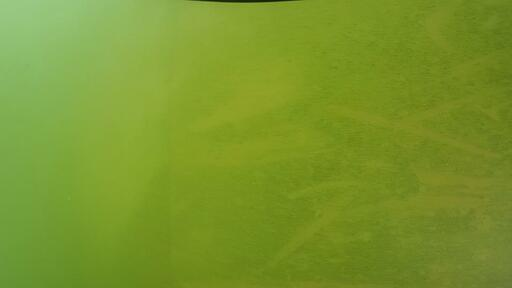}
         \includegraphics[width=\textwidth]{figures-video/day1-4.mkv/frames/paint_damaged/Frame-13761}
         \includegraphics[width=\textwidth]{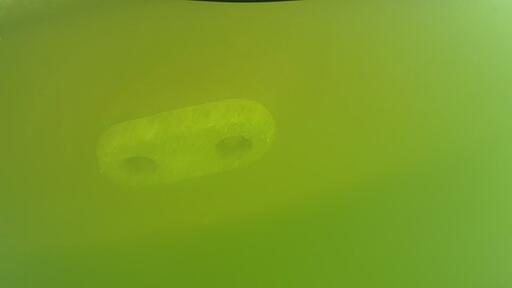}
     \end{subfigure}%
     \begin{subfigure}[b]{0.11\textwidth}
         \centering
         \includegraphics[width=\textwidth]{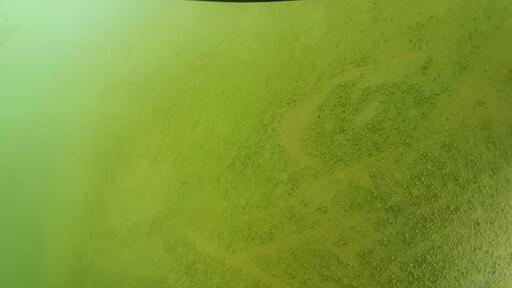}
         \includegraphics[width=\textwidth]{figures-video/day1-4.mkv/frames/paint_damaged/Frame-14094}
         \includegraphics[width=\textwidth]{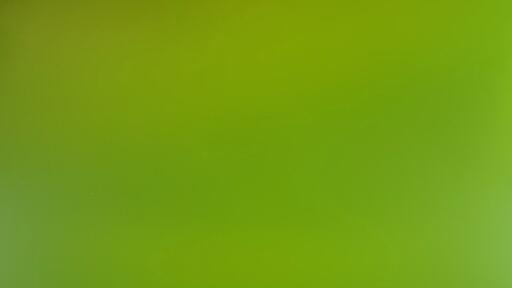}
     \end{subfigure}\\
     % ==================================================================================
     \begin{subfigure}[b]{1\textwidth}
         \centering
         \includegraphics[width=\textwidth]{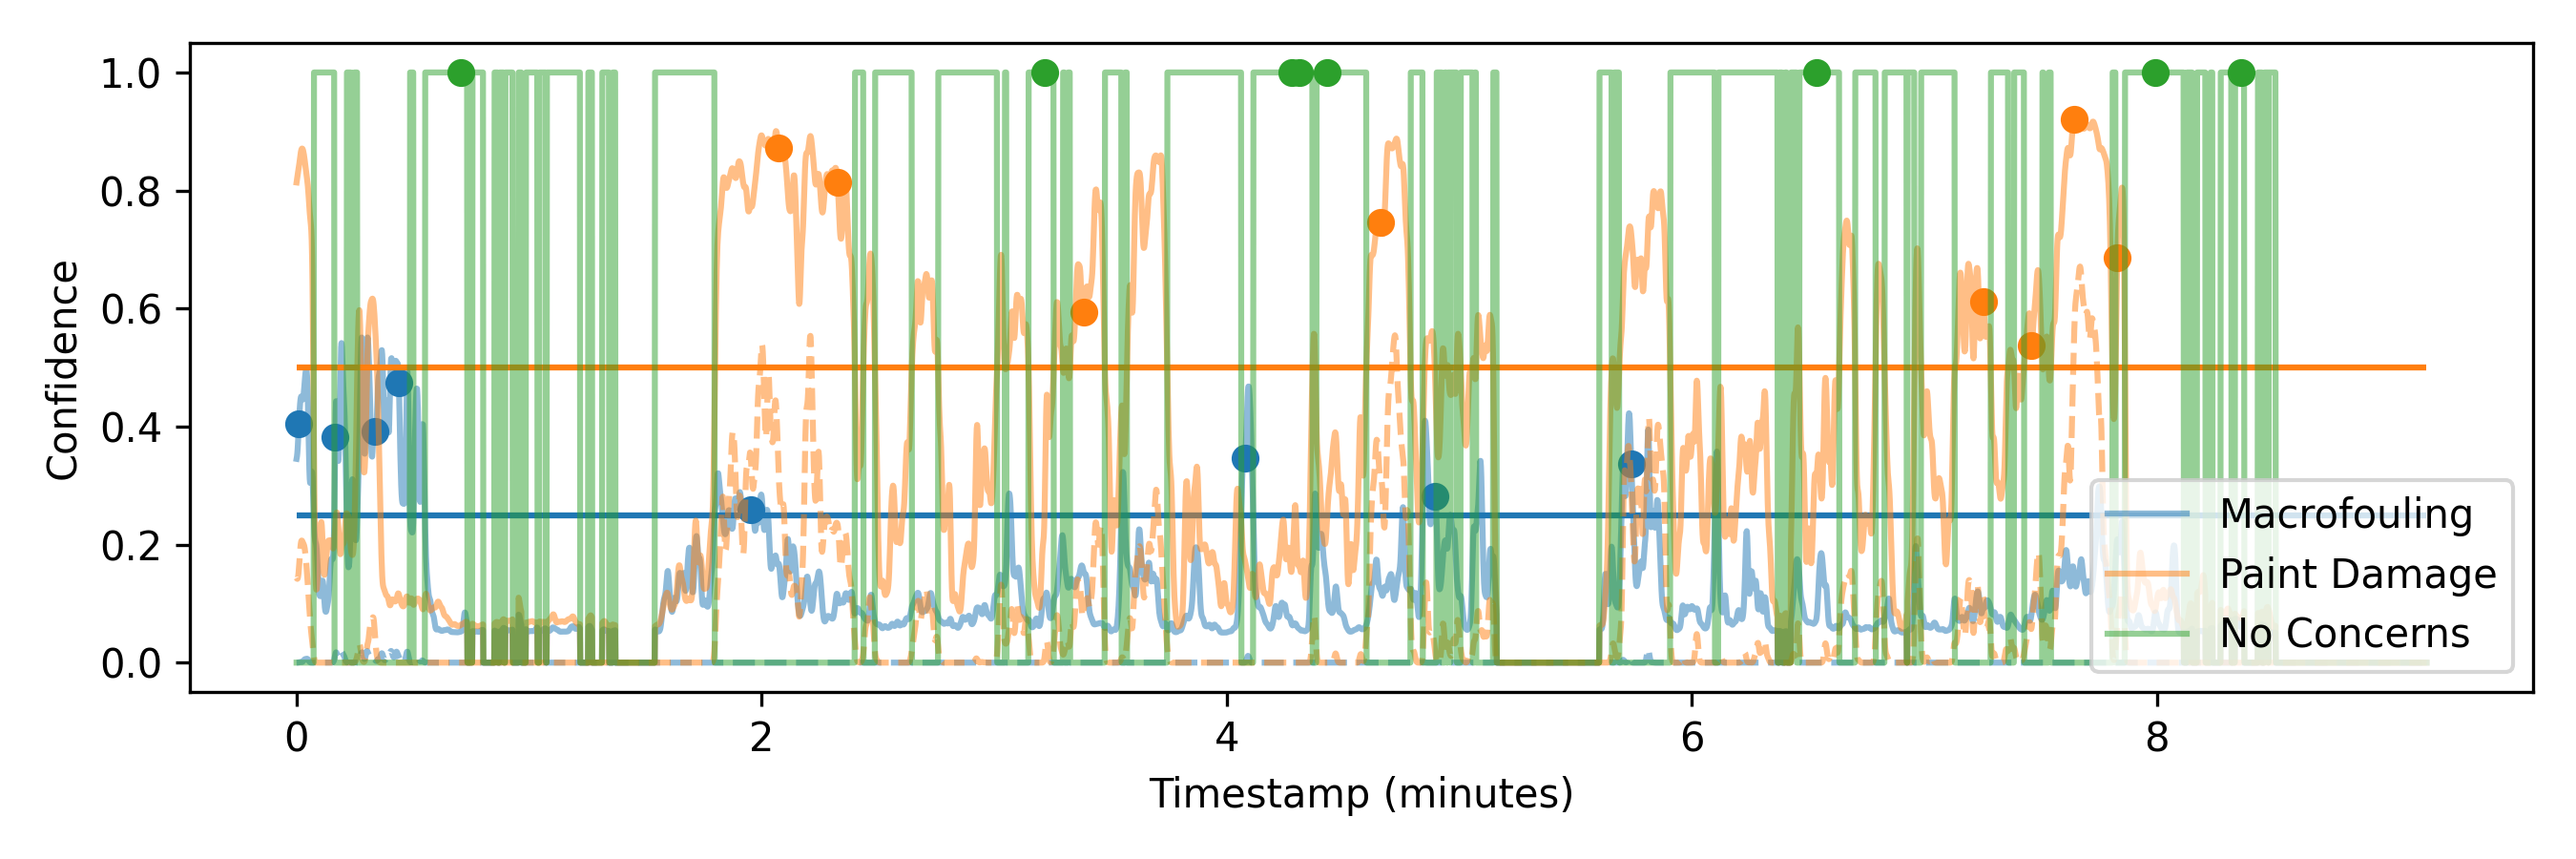}
     \end{subfigure}
        \caption[Analysis of ROV captured video with light fouling for macrofouling and paint damage using the ComFe model. ]{Analysis of ROV captured video with light fouling for macrofouling and paint damage using the ComFe model. The dots in the timeseries represent the frames shown above the plot, which are selected using the SKMPS method. The dashed lines represent the proportion of fouling or paint damage coverage predicted by the ComFe head, and the horizontal lines show the thresholds used to classify frames as having paint damage or macrofouling present.}
        \label{fig:prototype_examples}
\end{figure*}

% ==================================================================================================================================
\FloatBarrier
\newpage
\section{Detecting niche areas}
% ==================================================================================================================================

Due to small numbers of images of particular niche areas, such as discharges, ropeguards and anodes, we used upsampling when fitting models to detect niche areas. We also found the model that obtained best performance for identifying niches was prone to being confused by spurious features, and relied on visual inspection to select an initialisation where this confusion was minimized.

\begin{table*}[!h]
\caption[Brief summary of the 2021 cropped niche area dataset.]{Brief summary of the 2021 cropped niche area dataset. We show example training (first row) and testing (second row) images, and a table of the counts of each category in the dataset below. This dataset uses the same imagery as the 2021 cropped dataset, but with niche areas on recreational vessels removed as there was no fine-grained niche area data available in these cases. We trained models to identify anodes, circular features (plug, ropeguard and discharge) and gratings (Bow thruster and sea chest), and grouped the other categories into a \textit{no niche area present} super-category. For areas such as rudders, bilge keel and blockmarks, the images often appeared no different to a flat hull surface. }
\label{tbl:dataset_2023_cropped_niche}
\centering
\includegraphics[width=1\textwidth]{dataset_summary/nichearea_2021_cropped_training.jpg}
\includegraphics[width=1\textwidth]{dataset_summary/nichearea_2021_cropped_test.jpg}
\resizebox{\textwidth}{!}{%
\begin{tabular}[t]{lrrrrrrrrrrrr}
\toprule
\textbf{Category} & \textbf{Anode} & \textbf{Bilge keel} & \textbf{Blockmark} & \textbf{Bow thruster} & \textbf{Discharge} & \textbf{Hull} & \textbf{Plug} & \textbf{Prop} & \textbf{Ropeguard} & \textbf{Rudder} & \textbf{Sea chest grating} & \textbf{Total}  \\
\midrule
\textbf{Training}  & 65 & 420 & 469 & 402 & 34 & 5375 & 26 & 592 & 57 & 1051 & 525  & 9018  \\ 
\textbf{Test}  & 32  & 74     & 52  & 121& 16 & 209 & 18 & 60 & 30 & 93 & 136 & 841 \\ 
\bottomrule
\end{tabular}}
\end{table*}

\begin{figure*}[!b]
     \centering
     \begin{subfigure}[b]{0.3\textwidth}
         \centering
         \caption{Grating present}
         \label{fig:prototype_examples_pets_2}
         \includegraphics[width=\textwidth]{plots/2024_biofouling_prauc_niche_grating.png}
     \end{subfigure}%
     \begin{subfigure}[b]{0.3\textwidth}
         \centering
         \caption{Discharge/other present}
         \label{fig:prototype_examples_pets_2}
         \includegraphics[width=\textwidth]{plots/2024_biofouling_prauc_niche_discharge.png}
     \end{subfigure}%
     \begin{subfigure}[b]{0.3\textwidth}
         \centering
         \caption{Anode present}
         \label{fig:prototype_examples_pets_2}
         \includegraphics[width=\textwidth]{plots/2024_biofouling_prauc_niche_anode.png}
     \end{subfigure}
     \begin{subfigure}[b]{0.09\textwidth}
         % \caption{No vessel hull present}
         \picdims[height=4.5cm]{\textwidth}{3.5cm}{plots/2024_biofouling_prauc_legend.png}
         \vspace{1cm}
     \end{subfigure} \\
        \caption[Precision-recall curves for our best ComFe model for detecting the presence of fouling, paint damage and niche areas. ]{Precision-recall curves for our best ComFe model for detecting the presence of fouling, paint damage and niche areas, on the 2021 cropped test set. The models are trained using a ComFe head on the DINOv2 ViT-B/14 (f) w/reg backbone, using the 2021 cropped training data.}
        \label{fig:model_suite_average_precision}
\end{figure*}

\begin{figure*}[!b]
     \centering
     \begin{subfigure}[b]{0.12\textwidth}
         \centering
        \begin{overpic}[height=\textwidth, width=\textwidth]{example_images/1280px-HD_transparent_picture.png}
         \put (0,50) {\parbox{2cm}{\centering Input image}}
        \end{overpic}
        \begin{overpic}[height=\textwidth, width=\textwidth]{example_images/1280px-HD_transparent_picture.png}
         \put (0,50) {\parbox{2cm}{\centering Class\\prediction}}
        \end{overpic}
        % \begin{overpic}[height=\textwidth, width=\textwidth]{example_images/1280px-HD_transparent_picture.png}
        %  \put (0,50) {\parbox{2cm}{\centering Image\\prototypes}}
        % \end{overpic}
     \end{subfigure}
     \begin{subfigure}[b]{0.12\textwidth}
         \centering
         \caption{Hull}
         \label{fig:prototype_examples_planes_2}
         \includegraphics[width=\textwidth]{figures/niche/True_0_474_raw.jpg}
         \includegraphics[width=\textwidth]{figures/niche/True_0_474_class.jpg}
     \end{subfigure}
     \begin{subfigure}[b]{0.12\textwidth}
         \centering
         \caption{Grating}
         \label{fig:prototype_examples_pets_2}
         \includegraphics[width=\textwidth]{figures/niche/True_1_481_raw.jpg}
         \includegraphics[width=\textwidth]{figures/niche/True_1_481_class.jpg}
     \end{subfigure}
     \begin{subfigure}[b]{0.12\textwidth}
         \centering
         \caption{Grating}
         \label{fig:prototype_examples_planes_1}
         \includegraphics[width=\textwidth]{figures/niche/False_1_758_raw.jpg}
         \includegraphics[width=\textwidth]{figures/niche/False_1_758_class.jpg}
     \end{subfigure}
     \begin{subfigure}[b]{0.12\textwidth}
         \centering
         \caption{Anode}
         \label{fig:prototype_examples_cars_1}
         \includegraphics[width=\textwidth]{figures/niche/False_3_725_raw.jpg}
         \includegraphics[width=\textwidth]{figures/niche/False_3_725_class.jpg}
     \end{subfigure}
     \begin{subfigure}[b]{0.12\textwidth}
         \centering
         \caption{Discharge}
         \label{fig:prototype_examples_cars_2}
         \includegraphics[width=\textwidth]{figures/niche/False_2_539_raw.jpg}
         \includegraphics[width=\textwidth]{figures/niche/False_2_539_class.jpg}
     \end{subfigure}
     \begin{subfigure}[b]{0.12\textwidth}
         \centering
         \caption{Discharge}
         \label{fig:prototype_examples_pets_1}
         \includegraphics[width=\textwidth]{figures/niche/False_2_222_raw.jpg}
         \includegraphics[width=\textwidth]{figures/niche/False_2_222_class.jpg}
     \end{subfigure}
        \caption{Segmentation masks predicted by ComFe for the presence of niche areas.}
        \label{fig:salient_features_niches}
\end{figure*}

\begin{figure*}[!h]
     \centering
     \begin{subfigure}[b]{0.45\textwidth}
         \centering
         % \label{fig:prototype_examples_pets_2}
         \includegraphics[width=\textwidth]{figures-prototypes/niche/class_prototype_0.jpg}
         \caption{Hull}
     \end{subfigure}%
     \hfill{}
     \begin{subfigure}[b]{0.45\textwidth}
         \centering
         % \label{fig:prototype_examples_pets_2}
         \includegraphics[width=\textwidth]{figures-prototypes/niche/class_prototype_1.jpg}
         \caption{Grating}
     \end{subfigure}
     \begin{subfigure}[b]{0.45\textwidth}
         \centering
         % \label{fig:prototype_examples_pets_2}
         \includegraphics[width=\textwidth]{figures-prototypes/niche/class_prototype_2.jpg}
         \caption{Discharge/Other}
     \end{subfigure}
     \hfill{}
     \begin{subfigure}[b]{0.45\textwidth}
         \centering
         % \label{fig:prototype_examples_pets_2}
         \includegraphics[width=\textwidth]{figures-prototypes/niche/class_prototype_3.jpg}
         \caption{Anode}
     \end{subfigure}
        \caption{Predicted coverage within an image of fouling and paint damage by ComFe versus label categories for fouling and paint damage severity. }
        \label{fig:severity_coverage}
\end{figure*}

\begin{figure*}[!h]
     \centering
     \begin{subfigure}[b]{0.11\textwidth}
         \centering
        \begin{overpic}[height=0.5700\textwidth, width=\textwidth]{example_images/1280px-HD_transparent_picture.png}
         \put (0,20) {\parbox{1.5cm}{\centering \small Discharge\\Other}}
        \end{overpic}
        \begin{overpic}[height=0.5700\textwidth, width=\textwidth]{example_images/1280px-HD_transparent_picture.png}
         \put (0,20) {\parbox{1.5cm}{\centering \small No Niche}}
        \end{overpic}
     \end{subfigure}%
     \begin{subfigure}[b]{0.11\textwidth}
         \centering
         \includegraphics[width=\textwidth]{figures-video/day1-2.mkv/frames/niche_discharge_hole/Frame-1413}
         \includegraphics[width=\textwidth]{figures-video/day1-2.mkv/frames/no_niche/Frame-57}
     \end{subfigure}%
     \begin{subfigure}[b]{0.11\textwidth}
         \centering
         \includegraphics[width=\textwidth]{figures-video/day1-2.mkv/frames/niche_discharge_hole/Frame-1479}
         \includegraphics[width=\textwidth]{figures-video/day1-2.mkv/frames/no_niche/Frame-3498}     
     \end{subfigure}%
     \begin{subfigure}[b]{0.11\textwidth}
         \centering
         \includegraphics[width=\textwidth]{figures-video/day1-2.mkv/frames/niche_discharge_hole/Frame-1491}
         \includegraphics[width=\textwidth]{figures-video/day1-2.mkv/frames/no_niche/Frame-5433}
     \end{subfigure}%
     \begin{subfigure}[b]{0.11\textwidth}
         \centering
         \includegraphics[width=\textwidth]{figures-video/day1-2.mkv/frames/niche_discharge_hole/Frame-11589}
         \includegraphics[width=\textwidth]{figures-video/day1-2.mkv/frames/no_niche/Frame-6672}
     \end{subfigure}%
     \begin{subfigure}[b]{0.11\textwidth}
         \centering
         \includegraphics[width=\textwidth]{figures-video/day1-2.mkv/frames/niche_discharge_hole/Frame-11646}
         \includegraphics[width=\textwidth]{figures-video/day1-2.mkv/frames/no_niche/Frame-7689}
     \end{subfigure}%
     \begin{subfigure}[b]{0.11\textwidth}
         \centering
         \includegraphics[width=\textwidth]{figures-video/day1-2.mkv/frames/niche_discharge_hole/Frame-11715}
         \includegraphics[width=\textwidth]{figures-video/day1-2.mkv/frames/no_niche/Frame-9963}
     \end{subfigure}%
     \begin{subfigure}[b]{0.11\textwidth}
         \centering
         \includegraphics[width=\textwidth]{figures-video/day1-2.mkv/frames/niche_discharge_hole/Frame-11775}
         \includegraphics[width=\textwidth]{figures-video/day1-2.mkv/frames/no_niche/Frame-12618}
     \end{subfigure}%
     \begin{subfigure}[b]{0.11\textwidth}
         \centering
         \includegraphics[width=\textwidth]{figures-video/day1-2.mkv/frames/niche_discharge_hole/Frame-11883}
         \includegraphics[width=\textwidth]{figures-video/day1-2.mkv/frames/no_niche/Frame-14130}
     \end{subfigure}\\
     % ==================================================================================
     \begin{subfigure}[b]{1\textwidth}
         \centering
         \includegraphics[width=\textwidth]{figures-video/day1-2.mkv/plots/hull_category_all-plot-smoothed.png}
     \end{subfigure}
        \caption[Analysis of ROV captured video for niche areas using the ComFe model.]{Analysis of ROV captured video for niche areas using the ComFe model. The dots in the timeseries represent the frames shown above the plot, which are selected using the SKMPS method. The horizontal line shows the threshold used to classify frames as having a niche area present.}
        \label{fig:video_trial_examples_niche_discharge}
\end{figure*}

% Anodes
\begin{figure*}[!h]
     \centering
     \begin{subfigure}[b]{0.11\textwidth}
         \centering
        \begin{overpic}[height=0.5700\textwidth, width=\textwidth]{example_images/1280px-HD_transparent_picture.png}
         \put (0,20) {\parbox{1.5cm}{\centering \small Anode}}
        \end{overpic}
        \begin{overpic}[height=0.5700\textwidth, width=\textwidth]{example_images/1280px-HD_transparent_picture.png}
         \put (0,20) {\parbox{1.5cm}{\centering \small Discharge\\Other}}
        \end{overpic}
        \begin{overpic}[height=0.5700\textwidth, width=\textwidth]{example_images/1280px-HD_transparent_picture.png}
         \put (0,20) {\parbox{1.5cm}{\centering \small Grating}}
        \end{overpic}
        \begin{overpic}[height=0.5700\textwidth, width=\textwidth]{example_images/1280px-HD_transparent_picture.png}
         \put (0,20) {\parbox{1.5cm}{\centering \small No Niche}}
        \end{overpic}
     \end{subfigure}%
     \begin{subfigure}[b]{0.11\textwidth}
         \centering
         \includegraphics[width=\textwidth]{figures-video/day1-4.mkv/frames/niche_anode/Frame-180}
         \includegraphics[width=\textwidth]{figures-video/day1-4.mkv/frames/niche_discharge_hole/Frame-117}
         \includegraphics[width=\textwidth]{figures-video/day1-4.mkv/frames/niche_grating/Frame-8787}
         \includegraphics[width=\textwidth]{figures-video/day1-4.mkv/frames/no_niche/Frame-1272}
     \end{subfigure}%
     \begin{subfigure}[b]{0.11\textwidth}
         \centering
         \includegraphics[width=\textwidth]{figures-video/day1-4.mkv/frames/niche_anode/Frame-198}
         \includegraphics[width=\textwidth]{figures-video/day1-4.mkv/frames/niche_discharge_hole/Frame-213}
         \includegraphics[width=\textwidth]{figures-video/day1-4.mkv/frames/niche_grating/Frame-8790}
         \includegraphics[width=\textwidth]{figures-video/day1-4.mkv/frames/no_niche/Frame-4332}
     \end{subfigure}%
     \begin{subfigure}[b]{0.11\textwidth}
         \centering
         \includegraphics[width=\textwidth]{figures-video/day1-4.mkv/frames/niche_anode/Frame-237}
         \includegraphics[width=\textwidth]{figures-video/day1-4.mkv/frames/niche_discharge_hole/Frame-606}
         \includegraphics[width=\textwidth]{figures-video/day1-4.mkv/frames/niche_grating/Frame-8796}
         \includegraphics[width=\textwidth]{figures-video/day1-4.mkv/frames/no_niche/Frame-5793}
     \end{subfigure}%
     \begin{subfigure}[b]{0.11\textwidth}
         \centering
         \includegraphics[width=\textwidth]{figures-video/day1-4.mkv/frames/niche_anode/Frame-279}
         \includegraphics[width=\textwidth]{figures-video/day1-4.mkv/frames/niche_discharge_hole/Frame-723}
         \includegraphics[width=\textwidth]{figures-video/day1-4.mkv/frames/niche_grating/Frame-8799}
         \includegraphics[width=\textwidth]{figures-video/day1-4.mkv/frames/no_niche/Frame-7701}
     \end{subfigure}%
     \begin{subfigure}[b]{0.11\textwidth}
         \centering
         \includegraphics[width=\textwidth]{figures-video/day1-4.mkv/frames/niche_anode/Frame-345}
         \includegraphics[width=\textwidth]{figures-video/day1-4.mkv/frames/niche_discharge_hole/Frame-14298}
         \includegraphics[width=\textwidth]{figures-video/day1-4.mkv/frames/niche_grating/Frame-8802}
         \includegraphics[width=\textwidth]{figures-video/day1-4.mkv/frames/no_niche/Frame-8910}
     \end{subfigure}%
     \begin{subfigure}[b]{0.11\textwidth}
         \centering
         \includegraphics[width=\textwidth]{figures-video/day1-4.mkv/frames/niche_anode/Frame-405}
         \includegraphics[width=\textwidth]{figures-video/day1-4.mkv/frames/niche_discharge_hole/Frame-14343}
         \includegraphics[width=\textwidth]{figures-video/day1-4.mkv/frames/niche_grating/Frame-8805}
         \includegraphics[width=\textwidth]{figures-video/day1-4.mkv/frames/no_niche/Frame-11727}
     \end{subfigure}%
     \begin{subfigure}[b]{0.11\textwidth}
         \centering
         \includegraphics[width=\textwidth]{figures-video/day1-4.mkv/frames/niche_anode/Frame-447}
         \includegraphics[width=\textwidth]{figures-video/day1-4.mkv/frames/niche_discharge_hole/Frame-14478}
         \includegraphics[width=\textwidth]{figures-video/day1-4.mkv/frames/niche_grating/Frame-8808}
         \includegraphics[width=\textwidth]{figures-video/day1-4.mkv/frames/no_niche/Frame-13941}
     \end{subfigure}%
     \begin{subfigure}[b]{0.11\textwidth}
         \centering
         \includegraphics[width=\textwidth]{figures-video/day1-4.mkv/frames/niche_anode/Frame-498}
         \includegraphics[width=\textwidth]{figures-video/day1-4.mkv/frames/niche_discharge_hole/Frame-14535}
         \includegraphics[width=\textwidth]{figures-video/day1-4.mkv/frames/niche_grating/Frame-8811}
         \includegraphics[width=\textwidth]{figures-video/day1-4.mkv/frames/no_niche/Frame-15051}
     \end{subfigure}\\
     % ==================================================================================
     \begin{subfigure}[b]{1\textwidth}
         \centering
         \includegraphics[width=\textwidth]{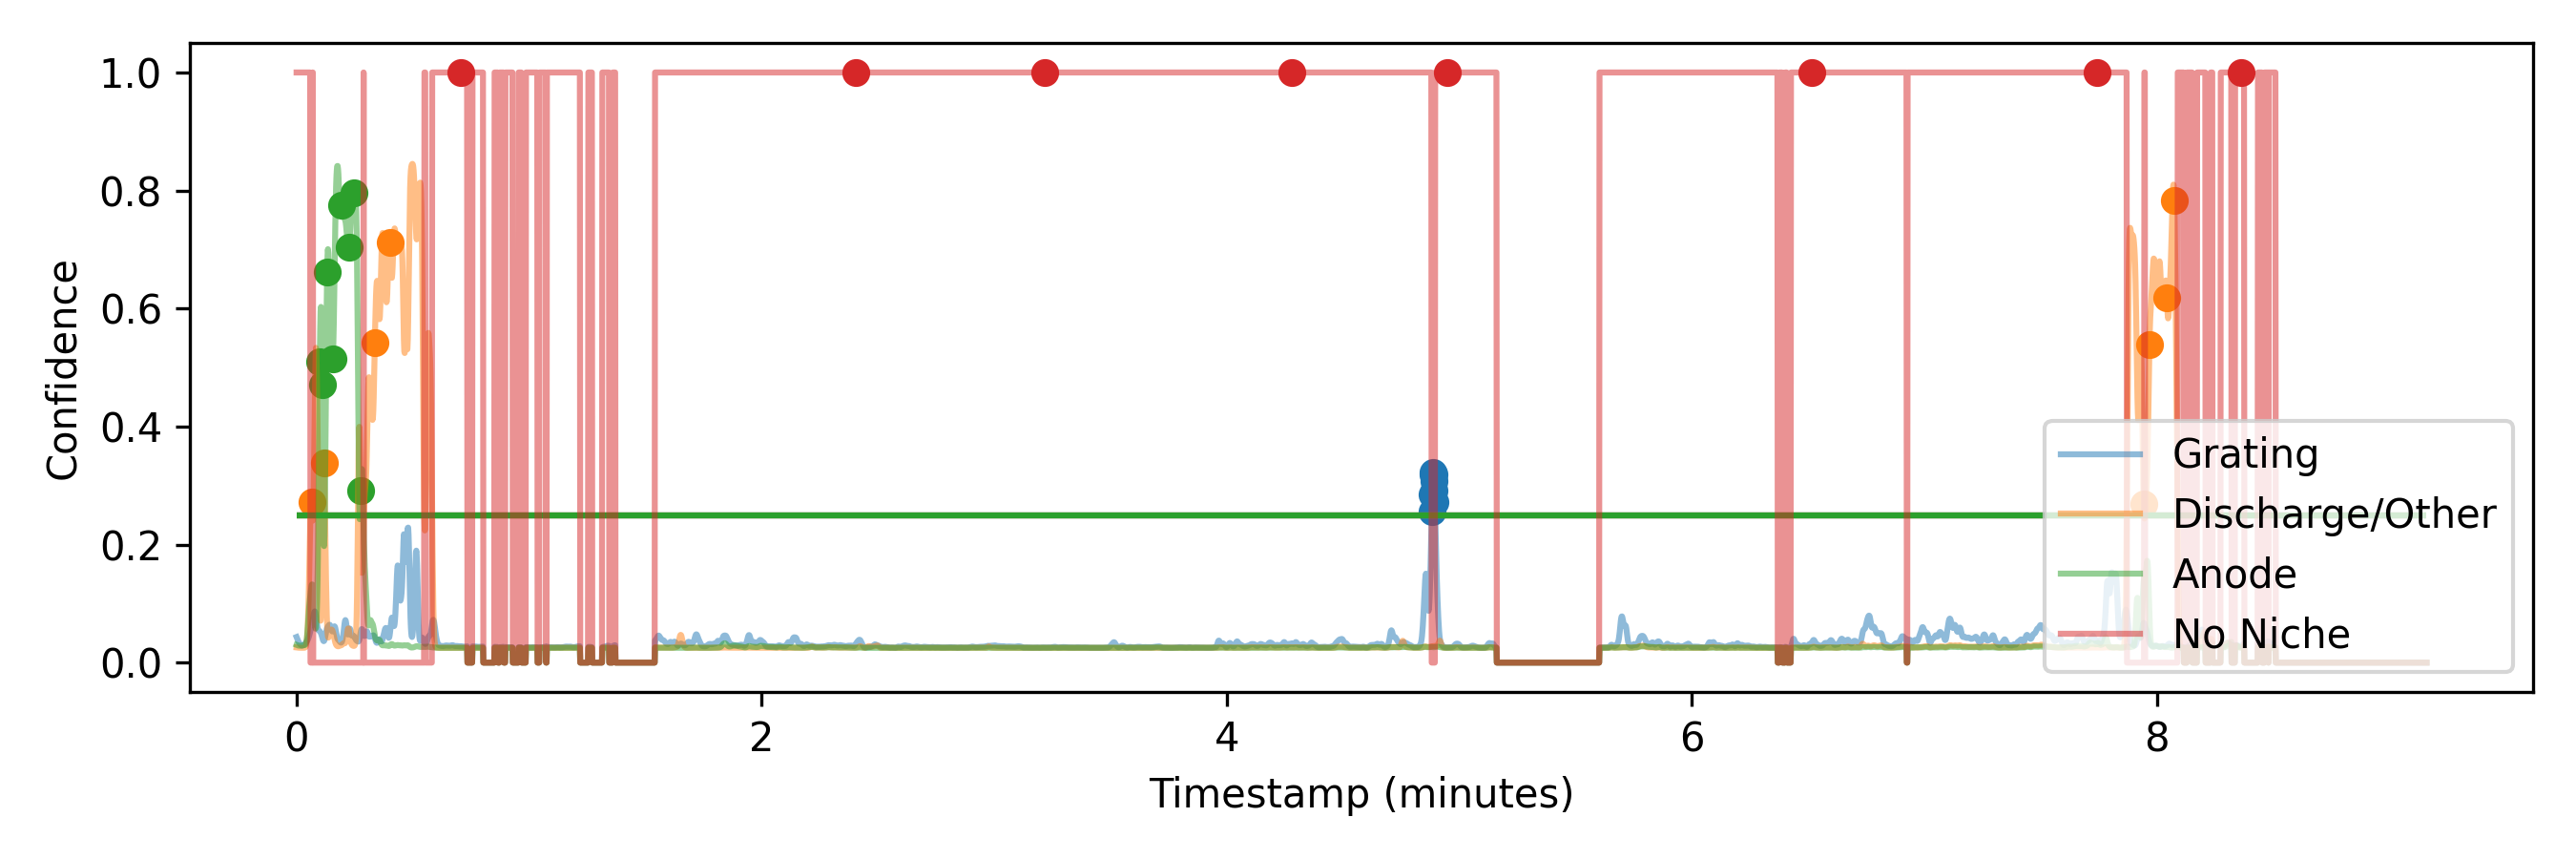}
     \end{subfigure}
        \caption[Analysis of ROV captured video for niche areas using the ComFe model.]{Analysis of ROV captured video for niche areas using the ComFe model. The dots in the timeseries represent the frames shown above the plot, which are selected using the SKMPS method. The horizontal line shows the threshold used to classify frames as having a niche area present.}
        \label{fig:prototype_examples}
\end{figure*}

% Sea chest
\begin{figure*}[!h]
     \centering
     \begin{subfigure}[b]{0.11\textwidth}
         \centering
        \begin{overpic}[height=0.5700\textwidth, width=\textwidth]{example_images/1280px-HD_transparent_picture.png}
         \put (0,20) {\parbox{1.5cm}{\centering \small Grating}}
        \end{overpic}
        \begin{overpic}[height=0.5700\textwidth, width=\textwidth]{example_images/1280px-HD_transparent_picture.png}
         \put (0,20) {\parbox{1.5cm}{\centering \small Anode}}
        \end{overpic}
        \begin{overpic}[height=0.5700\textwidth, width=\textwidth]{example_images/1280px-HD_transparent_picture.png}
         \put (0,20) {\parbox{1.5cm}{\centering \small No Niche}}
        \end{overpic}
     \end{subfigure}%
     \begin{subfigure}[b]{0.11\textwidth}
         \centering
         \includegraphics[width=\textwidth]{figures-video/day2-4.mkv/frames/niche_grating/Frame-939}
         \includegraphics[width=\textwidth]{figures-video/day2-4.mkv/frames/niche_anode/Frame-1149}
         \includegraphics[width=\textwidth]{figures-video/day2-4.mkv/frames/no_niche/Frame-3252}
     \end{subfigure}%
     \begin{subfigure}[b]{0.11\textwidth}
         \centering
         \includegraphics[width=\textwidth]{figures-video/day2-4.mkv/frames/niche_grating/Frame-1029.jpg}
         \includegraphics[width=\textwidth]{figures-video/day2-4.mkv/frames/niche_anode/Frame-1155}
         \includegraphics[width=\textwidth]{figures-video/day2-4.mkv/frames/no_niche/Frame-4857}
     \end{subfigure}%
     \begin{subfigure}[b]{0.11\textwidth}
         \centering
         \includegraphics[width=\textwidth]{figures-video/day2-4.mkv/frames/niche_grating/Frame-1842}
         \includegraphics[width=\textwidth]{figures-video/day2-4.mkv/frames/niche_anode/Frame-5922}
         \includegraphics[width=\textwidth]{figures-video/day2-4.mkv/frames/no_niche/Frame-5826}
     \end{subfigure}%
     \begin{subfigure}[b]{0.11\textwidth}
         \centering
         \includegraphics[width=\textwidth]{figures-video/day2-4.mkv/frames/niche_grating/Frame-2034}
         \includegraphics[width=\textwidth]{figures-video/day2-4.mkv/frames/niche_anode/Frame-5928}
         \includegraphics[width=\textwidth]{figures-video/day2-4.mkv/frames/no_niche/Frame-7239}
     \end{subfigure}%
     \begin{subfigure}[b]{0.11\textwidth}
         \centering
         \includegraphics[width=\textwidth]{figures-video/day2-4.mkv/frames/niche_grating/Frame-2355}
         \includegraphics[width=\textwidth]{figures-video/day2-4.mkv/frames/niche_anode/Frame-5937}
         \includegraphics[width=\textwidth]{figures-video/day2-4.mkv/frames/no_niche/Frame-8271}
     \end{subfigure}%
     \begin{subfigure}[b]{0.11\textwidth}
         \centering
         \includegraphics[width=\textwidth]{figures-video/day2-4.mkv/frames/niche_grating/Frame-2448}
         \includegraphics[width=\textwidth]{figures-video/day2-4.mkv/frames/niche_anode/Frame-5940}
         \includegraphics[width=\textwidth]{figures-video/day2-4.mkv/frames/no_niche/Frame-8859}
     \end{subfigure}%
     \begin{subfigure}[b]{0.11\textwidth}
         \centering
         \includegraphics[width=\textwidth]{figures-video/day2-4.mkv/frames/niche_grating/Frame-3861}
         \includegraphics[width=\textwidth]{figures-video/day2-4.mkv/frames/niche_anode/Frame-5949}
         \includegraphics[width=\textwidth]{figures-video/day2-4.mkv/frames/no_niche/Frame-10542}
     \end{subfigure}%
     \begin{subfigure}[b]{0.11\textwidth}
         \centering
         \includegraphics[width=\textwidth]{figures-video/day2-4.mkv/frames/niche_grating/Frame-3999}
         \includegraphics[width=\textwidth]{figures-video/day2-4.mkv/frames/niche_anode/Frame-5958}
         \includegraphics[width=\textwidth]{figures-video/day2-4.mkv/frames/no_niche/Frame-11604}
     \end{subfigure}\\
     % ==================================================================================
     \begin{subfigure}[b]{1\textwidth}
         \centering
         \includegraphics[width=\textwidth]{figures-video/day2-4.mkv/plots/hull_category_all-plot-smoothed.png}
     \end{subfigure}
        \caption[Analysis of ROV captured video for niche areas using the ComFe model.]{Analysis of ROV captured video for niche areas using the ComFe model.  The dots in the timeseries represent the frames shown above the plot, which are selected using the SKMPS method. The horizontal line shows the threshold used to classify frames as having a niche area present.}
        \label{fig:prototype_examples}
\end{figure*}
